# Supplementary material for: SmartPM: Automatic Adaptation of Dynamic Processes at Run-Time
Source: arXiv:1810.06374 source file (2018-10-12)
Supplement: Supplementary file 1 [file BPMNtoIndiGolog.tex]

\chapter{BPMN to \indigolog}
\label{bpmn-to-indigolog}

\begin{scriptsize}
\begin{alltt}
\textbf{\underline{BPMN Annotations :}}
\emph{Participant = \{act1,act2,act3,act4,rb1,rb2\}}

\textbf{\underline{Indigolog :}}
service(S) :- domain(S,[\textbf{\emph{act1,act2,act3,act4,rb1,rb2}}]).

\textbf{\underline{BPMN Annotations :}}
\emph{Capability = \{movement,hatchet,camera,gprs,extinguisher,battery,digger,powerpack\}}

\textbf{\underline{Indigolog :}}
capability(B) :- domain(B,[\textbf{\emph{movement,hatchet,camera,gprs,extinguisher,battery,digger,powerpack}}]).
\end{alltt}
\end{scriptsize}

\begin{scriptsize}
\begin{alltt}
\textbf{\underline{BPMN Annotations :}}
\textbf{\emph{Location_type = \{loc00,loc10,loc20,loc30,loc01,loc11,loc02,loc03,loc13,loc23,loc31,\\loc32,loc33\}}}

\textbf{\underline{Indigolog :}}
location_type(B) :- domain(B,[\textbf{\emph{loc00,loc10,loc20,loc30,loc01,loc11,loc02,loc03,loc13,loc23,loc31,\\loc32,loc33}}]).
\end{alltt}
\end{scriptsize}

\begin{scriptsize}
\begin{alltt}
\textbf{\underline{BPMN Annotations :}}
\textbf{\emph{Status_type = \{ok,fire,debris\}}}

\textbf{\underline{Indigolog :}}
status_type(B) :- domain(B,[\textbf{\emph{ok,fire,debris}}]).
\end{alltt}
\end{scriptsize}

In Indigolog, the domains representing boolean and integer types are already pre-defined.
\begin{scriptsize}
\begin{alltt}
\textbf{\underline{Indigolog :}}

boolean_type(Q).

integer_type(N).
\end{alltt}
\end{scriptsize}

\begin{scriptsize}
\begin{alltt}
\textbf{\underline{BPMN Annotations :}}
provides[prt:Participant,cap:Capability] = (bool:Boolean\_type)
\end{alltt}
\end{scriptsize}

\begin{scriptsize}
\begin{alltt}
\textbf{\underline{BPMN Annotations :}}
requires[task:Task,cap:Capability] = (bool:Boolean\_type)
\end{alltt}
\end{scriptsize}

\begin{scriptsize}
\begin{alltt}
\textbf{\underline{BPMN Annotations :}}

\textbf{\underline{Relevant for Adaptation :}}
\textbf{\emph{at[prt:Participant] = (loc:Location_type)}}
\textbf{\emph{evacuated[loc:Location_type] = (bool:Boolean\_type)}}
\textbf{\emph{status[loc:Location_type] = (st:Status_type)}}

\textbf{\underline{Not Relevant for Adaptation :}}
\textbf{\emph{batteryLevel[prt:Participant] = (int:Integer\_type)}}
\textbf{\emph{photoTaken[loc:Location_type] = (int:Integer\_type)}}
\textbf{\emph{generalBattery[] = (int:Integer\_type)}}
\textbf{\emph{batteryRecharging[] = (int:Integer\_type)}}
\textbf{\emph{moveStep[] = (int:Integer\_type)}}
\textbf{\emph{debrisStep[] = (int:Integer\_type)}}

\textbf{\underline{Indigolog :}}

\textbf{\emph{fun_fluent(at(SRVC)) :- service(SRVC).
fun_fluent(at_exp(SRVC)) :- service(SRVC).
fun_fluent(evacuated(LOC)) :- location_type(LOC).
fun_fluent(evacuated_exp(LOC)) :- location_type(LOC).
fun_fluent(status(LOC)) :- location_type(LOC).
fun_fluent(status_exp(LOC)) :- location_type(LOC).

fun_fluent(batteryLevel(SRVC)) :- service(SRVC).
fun_fluent(photoTaken(LOC)) :- location_type(LOC).
fun_fluent(generalBattery).
fun_fluent(batteryRecharging).
fun_fluent(moveStep).
fun_fluent(debrisStep).
}}
\end{alltt}
\end{scriptsize}
Si noti che ogni atomic term \textbf{relevant} deve essere convertito in una coppia di fluenti Indigolog, per memorizzare rispettivamente i valori reali e i valori attesi riguardanti le proprietà contestuali dello scenario. Perciò per ogni atomic term relevant definito nelle annotazioni XML, avremo un \textbf{fluente fisico} e uno \textbf{atteso}. Un fluente è un predicato il cui valore può essere modificato al termine di ogni azione. Al contrario, un ``classico'' predicato della logica del primo ordine è ``a-temporale'', cioè mantiene lo stesso valore per tutta la durata del programma. Si noti inoltre che nella definizione di un fluente non è richiesto di conoscere il tipo di dato che sarà memorizzato dentro il fluente stesso, ma il dominio di tutti gli argomenti che caratterizzeranno il fluente.

Al contrario, ogni atomic term "not relevant" sarà convertito in un singolo fluente fisico.
