# Supplementary material for: SmartPM: Automatic Adaptation of Dynamic Processes at Run-Time
Source: arXiv:1810.06374 source file (2018-10-12)
Supplement: Supplementary file 2 [file BPMNtoPDDL.tex]

\chapter{BPMN to PDDL}
\label{bpmn-to-pddl}
